# Supplementary material for: CVE-driven Attack Technique Prediction with Semantic Information Extraction and a Domain-specific Language Model
Source: arXiv:2309.02785 source file (2023-09-06)
Supplement: Supplementary file 1 [file Appendix_long.tex]

\bgroup

\begin{small}
\fontsize{9}{11}\selectfont
\begin{longtable}{|p{0.5cm}|p{4cm}|p{8cm}|} 
\hline

% \centering
\multicolumn{2}{|c}{\textbf{CVE Description}} &\\ 
\hline
%  & \textbf{Functionality} & \textbf{Predicted} \\ 
\multicolumn{2}{|p{5cm}|}{\textbf{Functionality}} & \textbf{Predicted} \\ 

\hline
\hline
1 & \multicolumn{2}{p{13cm}|}{CVE-2020-5250:  In PrestaShop before version 1.7.6.4, when a customer edits their address, they can freely change the id\_address in the form, and thus steal someone else's address. It is the same with CustomerForm, you are able to change the id\_customer and change all information of all accounts. The problem is patched in version 1.7.6.4.} \\ 
\hline
\multicolumn{2}{|p{5cm}|}{\begin{tabular}[c]{@{}l@{}}Password Reset\\Modify Configuration\end{tabular}} & \begin{tabular}[c]{@{}l@{}}\textbf{Password Reset:	7.1}\\\textbf{Modify Configuration:	1.21}\end{tabular} \\ 
\hline
2 & \multicolumn{2}{p{13cm}|}{CVE-2020-15170: apollo-adminservice before version 1.7.1 does not implement access controls. If users expose apollo-adminservice to internet(which is not recommended), there are potential security issues since apollo-adminservice is designed to work in intranet and it doesn't have access control built-in. Malicious hackers may access apollo-adminservice apis directly to access/edit the application's configurations. To fix the potential issue without upgrading, simply follow the advice that do not expose apollo-adminservice to internet.} \\ 
\hline
\multicolumn{2}{|p{5cm}|}{Modify Configuration} & \begin{tabular}[c]{@{}l@{}}Disable Protections:	8.32\\\textbf{Modify Configuration:	5.18}\end{tabular} \\ 
\hline
3 & \multicolumn{2}{p{13cm}|}{CVE-2020-5253:  NetHack before version 3.6.0 allowed malicious use of escaping of characters in the configuration file (usually .nethackrc) which could be exploited. This bug is patched in NetHack 3.6.0.} \\ 
\hline
\multicolumn{2}{|p{5cm}|}{Modify Configuration} & Modify Configuration:	11.27 \\ 
\hline
4 & \multicolumn{2}{p{13cm}|}{CVE-2020-5231:  In Opencast before 7.6 and 8.1, users with the role ROLE\_COURSE\_ADMIN can use the user-utils endpoint to create new users not including the role ROLE\_ADMIN. ROLE\_COURSE\_ADMIN is a non-standard role in Opencast which is referenced neither in the documentation nor in any code (except for tests) but only in the security configuration. From the name – implying an admin for a specific course – users would never expect that this role allows user creation. This issue is fixed in 7.6 and 8.1 which both ship a new default security configuration.} \\ 
\hline
\multicolumn{2}{|p{5cm}|}{Create Account} & \textbf{Create Account:	12.3} \\ 
\hline
5 & \multicolumn{2}{p{13cm}|}{CVE-2013-6129: The install/upgrade.php scripts in vBulletin 4.1 and 5 allow remote attackers to create administrative accounts via the customerid, htmldata[password], htmldata[confirmpassword], and htmldata[email] parameters, as exploited in the wild in October 2013.} \\ 
\hline
\multicolumn{2}{|p{5cm}|}{Create Account} & \textbf{Create Account:	13.84} \\ 
\hline
6 & \multicolumn{2}{p{13cm}|}{CVE-2015-4051:  Beckhoff IPC Diagnostics before 1.8 does not properly restrict access to functions in /config, which allows remote attackers to cause a denial of service (reboot or shutdown), create arbitrary users, or possibly have unspecified other impact via a crafted request, as demonstrated by a beckhoff.com:service:cxconfig:1\#Write SOAP action to /upnpisapi.} \\ 
\hline
\multicolumn{2}{|p{5cm}|}{\begin{tabular}[c]{@{}l@{}}Restart Or Reboot\\Create Account\end{tabular}} & \begin{tabular}[c]{@{}l@{}}\textbf{Restart Or Reboot:	11.53}\\\textbf{Create Account:	5.49}\end{tabular} \\ 
\hline
7 & \multicolumn{2}{p{13cm}|}{CVE-2019-3758:  RSA Archer, versions prior to 6.6 P2 (6.6.0.2), contain an improper authentication vulnerability. The vulnerability allows sysadmins to create user accounts with insufficient credentials. Unauthenticated attackers could gain unauthorized access to the system using those accounts.} \\ 
\hline
\multicolumn{2}{|p{5cm}|}{Create Account} & \textbf{Create Account:	10.56} \\ 
\hline
8 & \multicolumn{2}{p{13cm}|}{CVE-2019-3798:  Cloud Foundry Cloud Controller API Release, versions prior to 1.79.0, contains improper authentication when validating user permissions. A remote authenticated malicious user with the ability to create UAA clients and knowledge of the email of a victim in the foundation may escalate their privileges to that of the victim by creating a client with a name equal to the guid of their victim.}  \\ 
\hline
\multicolumn{2}{|p{5cm}|}{Create Account} & \textbf{Create Account:	11.43} \\ 
\hline
9 & \multicolumn{2}{p{13cm}|}{CVE-2019-18581:  Dell EMC Data Protection Advisor versions 6.3, 6.4, 6.5, 18.2 versions prior to patch 83, and 19.1 versions prior to patch 71 contain a server missing authorization vulnerability in the REST API. A remote authenticated malicious user with administrative privileges may potentially exploit this vulnerability to alter the application’s allowable list of OS commands. This may lead to arbitrary OS command execution as the regular user runs the DPA service on the affected system.} \\ 
\hline
\multicolumn{2}{|p{5cm}|}{Disable protections} & \textbf{Disable Protections:	7.47} \\ 
\hline
10 & \multicolumn{2}{p{13cm}|}{CVE-2018-17908:  WebAccess Versions 8.3.2 and prior. During installation, the application installer disables user access control and does not re-enable it after the installation is complete. This could allow an attacker to run elevated arbitrary code.} \\ 
\hline
\multicolumn{2}{|p{5cm}|}{Disable protections} & \begin{tabular}[c]{@{}l@{}}Install App:	10.31\\\textbf{Disable Protections:	2.81}\end{tabular} \\ 
\hline
11 & \multicolumn{2}{p{13cm}|}{CVE-2018-17892: NUUO CMS all versions 3.1 and prior, The application implements a method of user account control that causes standard account security features to not be utilized as intended, which could allow user account compromise and may allow for remote code execution.} \\ 
\hline
\multicolumn{2}{|p{5cm}|}{Disable protections} & \begin{tabular}[c]{@{}l@{}}Obtain Sensitive Information: Credentials:	8.02\\\textbf{Disable Protections:	1.82}\end{tabular} \\ 
\hline
12 & \multicolumn{2}{p{13cm}|}{CVE-2018-15397:  A vulnerability in the implementation of Traffic Flow Confidentiality (TFC) over IPsec functionality in Cisco Adaptive Security Appliance (ASA) Software and Cisco Firepower Threat Defense (FTD) Software could allow an unauthenticated, remote attacker to cause an affected device to restart unexpectedly, resulting in a denial of service (DoS) condition. The vulnerability is due to an error that may occur if the affected software renegotiates the encryption key for an IPsec tunnel when certain TFC traffic is in flight. An attacker could exploit this vulnerability by sending a malicious stream of TFC traffic through an established IPsec tunnel on an affected device. A successful exploit could allow the attacker to cause a daemon process on the affected device to crash, which could cause the device to crash and result in a DoS condition.} \\ 
\hline
\multicolumn{2}{|p{5cm}|}{Restart/Reboot} & \textbf{Restart Or Reboot:	14.91} \\ 
\hline
13 & \multicolumn{2}{p{13cm}|}{CVE-2018-15397:  A vulnerability in the implementation of Traffic Flow Confidentiality (TFC) over IPsec functionality in Cisco Adaptive Security Appliance (ASA) Software and Cisco Firepower Threat Defense (FTD) Software could allow an unauthenticated, remote attacker to cause an affected device to restart unexpectedly, resulting in a denial of service (DoS) condition. The vulnerability is due to an error that may occur if the affected software renegotiates the encryption key for an IPsec tunnel when certain TFC traffic is in flight. An attacker could exploit this vulnerability by sending a malicious stream of TFC traffic through an established IPsec tunnel on an affected device. A successful exploit could allow the attacker to cause a daemon process on the affected device to crash, which could cause the device to crash and result in a DoS condition.} \\ 
\hline
\multicolumn{2}{|p{5cm}|}{Restart/Reboot} & \textbf{Restart Or Reboot:	15.05} \\ 
\hline
14 & \multicolumn{2}{p{13cm}|}{CVE-2019-1817:  A vulnerability in the web proxy functionality of Cisco AsyncOS Software for Cisco Web Security Appliance could allow an unauthenticated, remote attacker to cause a denial of service (DoS) condition on an affected device. The vulnerability is due to improper validation of HTTP and HTTPS requests. An attacker could exploit this vulnerability by sending a malformed HTTP or HTTPS request to an affected device. An exploit could allow the attacker to cause a restart of the web proxy process, resulting in a temporary DoS condition.} \\ 
\hline
\multicolumn{2}{|p{5cm}|}{Restart/Reboot} & \textbf{Restart Or Reboot:	14.06} \\ 
\hline
15 & \multicolumn{2}{p{13cm}|}{CVE-2020-3312:  A vulnerability in the application policy configuration of Cisco Firepower Threat Defense (FTD) Software could allow an unauthenticated, remote attacker to gain unauthorized read access to sensitive data on an affected device. The vulnerability is due to insufficient application identification. An attacker could exploit this vulnerability by sending crafted traffic to an affected device. A successful exploit could allow the attacker to gain unauthorized read access to sensitive data.} \\ 
\hline
\multicolumn{2}{|p{5cm}|}{Obtain Sensitive Information: Other Data} & \textbf{Obtain Sensitive Information: Other Data:	8.7588} \\ 
\hline
16 & \multicolumn{2}{p{13cm}|}{CVE-2020-3477:  A vulnerability in the CLI parser of Cisco IOS Software and Cisco IOS XE Software could allow an authenticated, local attacker to access files from the flash: filesystem. The vulnerability is due to insufficient application of restrictions during the execution of a specific command. An attacker could exploit this vulnerability by using a specific command at the command line. A successful exploit could allow the attacker to obtain read-only access to files that are located on the flash: filesystem that otherwise might not have been accessible.} \\ 
\hline
\multicolumn{2}{|p{5cm}|}{Read Files, Obtain Sensitive Information: Other Data} & \begin{tabular}[c]{@{}l@{}}\textbf{Read Files:	9.47}\\\textbf{Obtain Sensitive Information: Other Data:	5.19}\end{tabular} \\ 
\hline
17 & \multicolumn{2}{p{13cm}|}{CVE-2019-15963:  A vulnerability in the web-based management interface of Cisco Unified Communications Manager could allow an authenticated, remote attacker to view sensitive information in the web-based management interface of the affected software. The vulnerability is due to insufficient protection of user-supplied input by the web-based management interface of the affected service. An attacker could exploit this vulnerability by accessing the interface and viewing restricted portions of the software configuration. A successful exploit could allow the attacker to gain access to sensitive information or conduct further attacks.} \\ 
\hline
\multicolumn{2}{|p{5cm}|}{Obtain Sensitive Information: Other Data} & \textbf{Obtain Sensitive Information: Other Data:	11.4} \\ 
\hline
18 & \multicolumn{2}{p{13cm}|}{CVE-2020-11045:  In FreeRDP after 1.0 and before 2.0.0, there is an out-of-bound read in in update\_read\_bitmap\_data that allows client memory to be read to an image buffer. The result displayed on screen as colour} \\ 
\hline
\multicolumn{2}{|p{5cm}|}{Read From Memory} & \textbf{Read From Memory:	7.54} \\ 
\hline
19 & \multicolumn{2}{p{13cm}|}{CVE-2018-7526:  In TotalAlert Web Application in BeaconMedaes Scroll Medical Air Systems prior to v4107600010.23, by accessing a specific uniform resource locator (URL) on the webserver, a malicious user may be able to access information in the application without authenticating.} \\ 
\hline
\multicolumn{2}{|p{5cm}|}{Obtain Sensitive Information: Other Data} & \textbf{Obtain Sensitive Information: Other Data:	9.89} \\ 
\hline
20 & \multicolumn{2}{p{13cm}|}{CVE-2018-5445:  A Path Traversal issue was discovered in Advantech WebAccess/SCADA versions prior to V8.2\_20170817. An attacker has read access to files within the directory structure of the target device.} \\ 
\hline
\multicolumn{2}{|p{5cm}|}{Read Files} & \textbf{Read Files:	13.55} \\ 
\hline
21 & \multicolumn{2}{p{13cm}|}{CVE-2018-18990:  LCDS Laquis SCADA prior to version 4.1.0.4150 allows a user-supplied path in file operations prior to proper validation. An attacker can leverage this vulnerability to disclose sensitive information under the context of the web server process.} \\ 
\hline
\multicolumn{2}{|p{5cm}|}{Obtain Sensitive Information: Other Data} & \textbf{Obtain Sensitive Information: Other Data:	10.04} \\ 
\hline
22 & \multicolumn{2}{p{13cm}|}{CVE-2020-16211:  Advantech WebAccess HMI Designer, Versions 2.1.9.31 and prior. An out-of-bounds read vulnerability may be exploited by processing specially crafted project files, which may allow an attacker to read information.} \\ 
\hline
\multicolumn{2}{|p{5cm}|}{\begin{tabular}[c]{@{}l@{}}Read Files\\Read From Memory\end{tabular}} & \begin{tabular}[c]{@{}l@{}}\textbf{Read Files:	7.61}\\\textbf{Read From Memory:	5.15}\end{tabular} \\ 
\hline
23 & \multicolumn{2}{p{13cm}|}{CVE-2020-11652:  An issue was discovered in SaltStack Salt before 2019.2.4 and 3000 before 3000.2. The salt-master process ClearFuncs class allows access to some methods that improperly sanitize paths. These methods allow arbitrary directory access to authenticated users.} \\ 
\hline
\multicolumn{2}{|p{5cm}|}{Obtain Sensitive Information: Other Data} & \begin{tabular}[c]{@{}l@{}}Obtain Sensitive Information: Credentials:	6.79\\\textbf{Obtain Sensitive Information: Other Data:	4.93}\end{tabular} \\ 
\hline
24 & \multicolumn{2}{p{13cm}|}{CVE-2017-16651:  Roundcube Webmail before 1.1.10, 1.2.x before 1.2.7, and 1.3.x before 1.3.3 allows unauthorized access to arbitrary files on the host's filesystem, including configuration files, as exploited in the wild in November 2017. The attacker must be able to authenticate at the target system with a valid username/password as the attack requires an active session. The issue is related to file-based attachment plugins and \_task=settings\_action=upload-display\_from=timezone requests.} \\ 
\hline
\multicolumn{2}{|p{5cm}|}{Read Files} & \textbf{Read Files:	12.42} \\ 
\hline
25 & \multicolumn{2}{p{13cm}|}{CVE-2019-5910:  Directory traversal vulnerability in HOUSE GATE App for iOS 1.7.8 and earlier allows remote attackers to read arbitrary files via unspecified vectors.} \\ 
\hline
\multicolumn{2}{|p{5cm}|}{Read Files} & \textbf{Read Files:	14.77} \\ 
\hline
26 & \multicolumn{2}{p{13cm}|}{CVE-2019-3787:  Cloud Foundry UAA, versions prior to 73.0.0, falls back to appending “unknown.org” to a user's email address when one is not provided and the user name does not contain an @ character. This domain is held by a private company, which leads to attack vectors including password recovery emails sent to a potentially fraudulent address. This would allow the attacker to gain complete control of the user's account.} \\ 
\hline
\multicolumn{2}{|p{5cm}|}{Obtain sensitive information: Credentials} & \textbf{Obtain Sensitive Information: Credentials:	7.69} \\ 
\hline
27 & \multicolumn{2}{p{13cm}|}{CVE-2019-3763:  The RSA Identity Governance and Lifecycle software and RSA Via Lifecycle and Governance products prior to 7.1.0 P08 contain an information exposure vulnerability. The Office 365 user password may get logged in a plain text format in the Office 365 connector debug log file. An authenticated malicious local user with access to the debug logs may obtain the exposed password to use in further attacks.} \\ 
\hline
\multicolumn{2}{|p{5cm}|}{Obtain sensitive information: Credentials} & \textbf{Obtain Sensitive Information: Credentials:	11.86} \\ 
\hline
28 & \multicolumn{2}{p{13cm}|}{CVE-2018-17900:  Yokogawa STARDOM Controllers FCJ, FCN-100, FCN-RTU, FCN-500, All versions R4.10 and prior, The web application improperly protects credentials which could allow an attacker to obtain credentials for remote access to controllers.} \\ 
\hline
\multicolumn{2}{|p{5cm}|}{Obtain sensitive information: Credentials} & \textbf{Obtain Sensitive Information: Credentials:	12.61} \\ 
\hline
29 & \multicolumn{2}{p{13cm}|}{CVE-2019-6549:  An attacker could retrieve plain-text credentials stored in a XML file on PR100088 Modbus gateway versions prior to Release R02 (or Software Version 1.1.13166) through FTP.} \\ 
\hline
\multicolumn{2}{|p{5cm}|}{Obtain sensitive information: Credentials} & \textbf{Obtain Sensitive Information: Credentials:	13.08} \\ 
\hline
30 & \multicolumn{2}{p{13cm}|}{CVE-2020-4408:  The IBM QRadar Advisor 1.1 through 2.5.2 with Watson App for IBM QRadar SIEM does not adequately mask all passwords during input, which could be obtained by a physical attacker nearby. IBM X-Force ID: 179536.} \\ 
\hline
\multicolumn{2}{|p{5cm}|}{Obtain sensitive information: Credentials} & \textbf{Obtain Sensitive Information: Credentials:	8.46} \\ 
\hline
31 & \multicolumn{2}{p{13cm}|}{CVE-2019-13922:  A vulnerability has been identified in SINEMA Remote Connect Server (All versions  V2.0 SP1). An attacker with administrative privileges can obtain the hash of a connected device's password. The security vulnerability could be exploited by an attacker with network access to the SINEMA Remote Connect Server and administrative privileges. At the time of advisory publication no public exploitation of this security vulnerability was known.} \\ 
\hline
\multicolumn{2}{|p{5cm}|}{Obtain sensitive information: Credentials} & \textbf{Obtain Sensitive Information: Credentials:	12.54} \\ 
\hline
32 & \multicolumn{2}{p{13cm}|}{CVE-2018-7259:  The FSX / P3Dv4 installer 2.0.1.231 for Flight Sim Labs A320-X sends a user's Google account credentials to http://installLog.flightsimlabs.com/LogHandler3.ashx if a pirated serial number has been entered, which allows remote attackers to obtain sensitive information, e.g., by sniffing the network for cleartext HTTP traffic. This behavior was removed in 2.0.1.232.} \\ 
\hline
\multicolumn{2}{|p{5cm}|}{Obtain sensitive information: Credentials} & \textbf{Obtain Sensitive Information: Credentials:	7.17} \\ 
\hline
33 & \multicolumn{2}{p{13cm}|}{CVE-2019-15956:  A vulnerability in the web management interface of Cisco AsyncOS Software for Cisco Web Security Appliance (WSA) could allow an authenticated, remote attacker to perform an unauthorized system reset on an affected device. The vulnerability is due to improper authorization controls for a specific URL in the web management interface. An attacker could exploit this vulnerability by sending a crafted HTTP request to an affected device. A successful exploit could have a twofold impact: the attacker could either change the administrator password, gaining privileged access, or reset the network configuration details, causing a denial of service (DoS) condition. In both scenarios, manual intervention is required to restore normal operations.} \\ 
\hline
\multicolumn{2}{|p{5cm}|}{\begin{tabular}[c]{@{}l@{}}Restart Or Reboot\\Password Reset\end{tabular}} & \begin{tabular}[c]{@{}l@{}}\textbf{Restart Or Reboot}:	11.48\\Modify Configuration:	3.96\\Delete Files:	2.32\\Install App:	1.66\\\textbf{Password Reset:	1.05}\end{tabular} \\ 
\hline
34 & \multicolumn{2}{p{13cm}|}{CVE-2019-1915:  A vulnerability in the web-based interface of Cisco Unified Communications Manager, Cisco Unified Communications Manager Session Management Edition (SME), Cisco Unified Communications Manager IM and Presence (Unified CM IMamp;P) Service, and Cisco Unity Connection could allow an unauthenticated, remote attacker to conduct a cross-site request forgery (CSRF) attack on an affected system. The vulnerability is due to insufficient CSRF protections by the affected software. An attacker could exploit this vulnerability by persuading a targeted user to click a malicious link. A successful exploit could allow the attacker to send arbitrary requests that could change the password of a targeted user. An attacker could then take unauthorized actions on behalf of the targeted user.} \\ 
\hline
\multicolumn{2}{|p{5cm}|}{Password Reset} & \textbf{Password Reset:	9.06} \\ 
\hline
35 & \multicolumn{2}{p{13cm}|}{CVE-2019-3775:  Cloud Foundry UAA, versions prior to v70.0, allows a user to update their own email address. A remote authenticated user can impersonate a different user by changing their email address to that of a different user.} \\ 
\hline
\multicolumn{2}{|p{5cm}|}{Password Reset} & \textbf{Password Reset:	12.08} \\ 
\hline
36 & \multicolumn{2}{p{13cm}|}{CVE-2019-3782:  Cloud Foundry CredHub CLI, versions prior to 2.2.1, inadvertently writes authentication credentials provided via environment variables to its persistent config file. A local authenticated malicious user with access to the CredHub CLI config file can use these credentials to retrieve and modify credentials stored in CredHub that are authorized to the targeted user.} \\ 
\hline
\multicolumn{2}{|p{5cm}|}{Password Reset} & \textbf{Password Reset:	8.88} \\ 
\hline
37 & \multicolumn{2}{p{13cm}|}{CVE-2019-3723:  Dell EMC OpenManage Server Administrator (OMSA) versions prior to 9.1.0.3 and prior to 9.2.0.4 contain a web parameter tampering vulnerability. A remote unauthenticated attacker could potentially manipulate parameters of web requests to OMSA to create arbitrary files with empty content or delete the contents of any existing file, due to improper input parameter validation} \\ 
\hline
\multicolumn{2}{|p{5cm}|}{\begin{tabular}[c]{@{}l@{}}Create Or Upload File\\Write To Existing File\\Delete Files\end{tabular}} & \begin{tabular}[c]{@{}l@{}}\textbf{Create Or Upload File:	9.58}\\\textbf{Write To Existing File:	5.9}\\\textbf{Delete Files:	5.49}\end{tabular} \\ 
\hline
38 & \multicolumn{2}{p{13cm}|}{CVE-2019-3750:  Dell Command Update versions prior to 3.1 contain an Arbitrary File Deletion Vulnerability. A local authenticated malicious user with low privileges potentially could exploit this vulnerability to delete arbitrary files by creating a symlink from the "Temp\textbackslash{}IC\textbackslash{}ICDebugLog.txt" to any targeted file. This issue occurs because of insecure handling of Temp directory permissions that were set incorrectly.} \\ 
\hline
\multicolumn{2}{|p{5cm}|}{Delete files} & \textbf{Delete Files:	13.84} \\ 
\hline
38 & \multicolumn{2}{p{13cm}|}{CVE-2020-1163:  An elevation of privilege vulnerability exists in Windows Defender that leads arbitrary file deletion on the system.To exploit the vulnerability, an attacker would first have to log on to the system, aka 'Microsoft Windows Defender Elevation of Privilege Vulnerability'. This CVE ID is unique from CVE-2020-1170.} \\ 
\hline
\multicolumn{2}{|p{5cm}|}{Delete files} & \textbf{Delete Files:	12.92} \\ 
\hline
40 & \multicolumn{2}{p{13cm}|}{CVE-2020-15189:  SOY CMS 3.0.2 and earlier is affected by Remote Code Execution (RCE) using Unrestricted File Upload. Cross-Site Scripting(XSS) vulnerability that was used in CVE-2020-15183 can be used to increase impact by redirecting the administrator to access a specially crafted page. This vulnerability is caused by insecure configuration in elFinder. This is fixed in version 3.0.2.328.} \\ 
\hline
\multicolumn{2}{|p{5cm}|}{Create/Upload file} & \textbf{Create Or Upload File:	13.11} \\ 
\hline
41 & \multicolumn{2}{p{13cm}|}{CVE-2020-5297:  In OctoberCMS (october/october composer package) versions from 1.0.319 and before 1.0.466, an attacker can exploit this vulnerability to upload jpg, jpeg, bmp, png, webp, gif, ico, css, js, woff, woff2, svg, ttf, eot, json, md, less, sass, scss, xml files to any directory of an October CMS server. The vulnerability is only exploitable by an authenticated backend user with the \`{}cms.manage\_assets\`{} permission. Issue has been patched in Build 466 (v1.0.466).} \\ 
\hline
\multicolumn{2}{|p{5cm}|}{Create/Upload file} & \textbf{Create Or Upload File:	15.2911} \\ 
\hline
42 & \multicolumn{2}{p{13cm}|}{CVE-2012-6081:  Multiple unrestricted file upload vulnerabilities in the (1) twikidraw (action/twikidraw.py) and (2) anywikidraw (action/anywikidraw.py) actions in MoinMoin before 1.9.6 allow remote authenticated users with write permissions to execute arbitrary code by uploading a file with an executable extension, then accessing it via a direct request to the file in an unspecified directory, as exploited in the wild in July 2012.} \\ 
\hline
\multicolumn{2}{|p{5cm}|}{Create/Upload file} & \textbf{Create Or Upload File:	14.87} \\ 
\hline
43 & \multicolumn{2}{p{13cm}|}{CVE-2011-4106:  TimThumb (timthumb.php) before 2.0 does not validate the entire source with the domain white list, which allows remote attackers to upload and execute arbitrary code via a URL containing a white-listed domain in the src parameter, then accessing it via a direct request to the file in the cache directory, as exploited in the wild in August 2011.} \\ 
\hline
\multicolumn{2}{|p{5cm}|}{Create/Upload file} & \textbf{Create Or Upload File:	12.71} \\ 
\hline
44 & \multicolumn{2}{p{13cm}|}{CVE-2016-3088:  The Fileserver web application in Apache ActiveMQ 5.x before 5.14.0 allows remote attackers to upload and execute arbitrary files via an HTTP PUT followed by an HTTP MOVE request.} \\ 
\hline
\multicolumn{2}{|p{5cm}|}{Create/Upload file} & \textbf{Create Or Upload File:	14.73} \\ 
\hline
45 & \multicolumn{2}{p{13cm}|}{CVE-2020-3476:  A vulnerability in the CLI implementation of a specific command of Cisco IOS XE Software could allow an authenticated, local attacker to overwrite arbitrary files in the underlying host file system. The vulnerability is due to insufficient validation of the parameters of a specific CLI command. An attacker could exploit this vulnerability by issuing that command with specific parameters. A successful exploit could allow the attacker to overwrite the content of any arbitrary file that resides on the underlying host file system.} \\ 
\hline
\multicolumn{2}{|p{5cm}|}{Write to existing file} & \textbf{Write To Existing File:	12.2} \\ 
\hline
46 & \multicolumn{2}{p{13cm}|}{CVE-2020-3440:  A vulnerability in Cisco Webex Meetings Desktop App for Windows could allow an unauthenticated, remote attacker to overwrite arbitrary files on an end-user system. The vulnerability is due to improper validation of URL parameters that are sent from a website to the affected application. An attacker could exploit this vulnerability by persuading a user to follow a URL to a website that is designed to submit crafted input to the affected application. A successful exploit could allow the attacker to overwrite arbitrary files on the affected system, possibly corrupting or deleting critical system files.} \\ 
\hline
\multicolumn{2}{|p{5cm}|}{Write to existing file} & \textbf{Write To Existing File:	12.54} \\ 
\hline
47 & \multicolumn{2}{p{13cm}|}{CVE-2019-1836:  A vulnerability in the system shell for Cisco Nexus 9000 Series Fabric Switches in Application Centric Infrastructure (ACI) mode could allow an authenticated, local attacker to use symbolic links to overwrite system files. These system files may be sensitive and should not be overwritable by non-root users. The attacker would need valid device credentials. The vulnerability is due to incorrect symbolic link verification of directory paths when they are used in the system shell. An attacker could exploit this vulnerability by authenticating to the device and providing crafted user input to specific symbolic link CLI commands. Successful exploitation could allow the attacker to overwrite system files that should be restricted. This vulnerability has been fixed in software version 14.1(1i).} \\ 
\hline
\multicolumn{2}{|p{5cm}|}{Write to existing file} & \textbf{Write To Existing File:	12.6} \\ 
\hline
48 & \multicolumn{2}{p{13cm}|}{CVE-2020-3237:  A vulnerability in the Cisco Application Framework component of the Cisco IOx application environment could allow an authenticated, local attacker to overwrite arbitrary files in the virtual instance that is running on the affected device. The vulnerability is due to insufficient path restriction enforcement. An attacker could exploit this vulnerability by including a crafted file in an application package. An exploit could allow the attacker to overwrite files.} \\ 
\hline
\multicolumn{2}{|p{5cm}|}{Write to existing file} & \textbf{Write To Existing File:	12.79} \\ 
\hline
49 & \multicolumn{2}{p{13cm}|}{CVE-2008-4996:  init in initramfs-tools 0.92f allows local users to overwrite arbitrary files via a symlink attack on the /tmp/initramfs.debug temporary file.} \\ 
\hline
\multicolumn{2}{|p{5cm}|}{Write to existing file} & \textbf{Write To Existing File:	11.4726} \\ 
\hline
50 & \multicolumn{2}{p{13cm}|}{CVE-2018-15392:  A vulnerability in the DHCP service of Cisco Industrial Network Director could allow an unauthenticated, adjacent attacker to cause a denial of service (DoS) condition. The vulnerability is due to improper handling of DHCP lease requests. An attacker could exploit this vulnerability by sending malicious DHCP lease requests to an affected application. A successful exploit could allow the attacker to cause the DHCP service to terminate, resulting in a DoS condition.} \\ 
\hline
\multicolumn{2}{|p{5cm}|}{Restart Or Reboot, Memory Read (Memory Errors)} & \begin{tabular}[c]{@{}l@{}}\textbf{Restart Or Reboot:	13.34}\\\textbf{Memory Read (Memory Errors):	2.77}\end{tabular} \\ 
\hline
51 & \multicolumn{2}{p{13cm}|}{CVE-2018-15392:  A vulnerability in the DHCP service of Cisco Industrial Network Director could allow an unauthenticated, adjacent attacker to cause a denial of service (DoS) condition. The vulnerability is due to improper handling of DHCP lease requests. An attacker could exploit this vulnerability by sending malicious DHCP lease requests to an affected application. A successful exploit could allow the attacker to cause the DHCP service to terminate, resulting in a DoS condition.} \\ 
\hline
\multicolumn{2}{|p{5cm}|}{Restart Or Reboot} & \textbf{Restart Or Reboot:	13.34} \\ 
\hline
52 & \multicolumn{2}{p{13cm}|}{CVE-2020-5210:  In NetHack before 3.6.5, an invalid argument to the -w command line option can cause a buffer overflow resulting in a crash or remote code execution/privilege escalation. This vulnerability affects systems that have NetHack installed suid/sgid and shared systems that allow users to influence command line options. Users should upgrade to NetHack 3.6.5.} \\ 
\hline
\multicolumn{2}{|p{5cm}|}{Memory Read (Memory Errors)} & \textbf{Memory Read (Memory Errors):	6.43} \\ 
\hline
53 & \multicolumn{2}{p{13cm}|}{CVE-2020-11019:  In FreeRDP less than or equal to 2.0.0, when running with logger set to "WLOG\_TRACE", a possible crash of application could occur due to a read of an invalid array index. Data could be printed as string to local terminal. This has been fixed in 2.1.0.} \\ 
\hline
\multicolumn{2}{|p{5cm}|}{Memory Read (Memory Errors)} & \begin{tabular}[c]{@{}l@{}}\textbf{Restart Or Reboot:	11.86}\\\textbf{Memory Read (Memory Errors):	2.35}\end{tabular} \\ 
\hline
54 & \multicolumn{2}{p{13cm}|}{CVE-2020-15137:  All versions of HoRNDIS are affected by an integer overflow in the RNDIS packet parsing routines. A malicious USB device can trigger disclosure of unrelated kernel memory to userspace applications on the host, or can cause the kernel to crash. Kernel memory disclosure is especially likely on 32-bit kernels; 64-bit kernels are more likely to crash on attempted exploitation. It is not believed that kernel memory corruption is possible, or that unattended kernel memory disclosure without the collaboration of a userspace program running on the host is possible. The vulnerability is in \`{}HoRNDIS::receivePacket\`{}. \`{}msg\_len\`{}, \`{}data\_ofs\`{}, and \`{}data\_len\`{} can be controlled by an attached USB device, and a negative value of \`{}data\_ofs\`{} can bypass the check for \`{}(data\_ofs + data\_len + 8)  msg\_len\`{}, and subsequently can cause a wild pointer copy in the \`{}mbuf\_copyback\`{} call. The software is not maintained and no patches are planned. Users of multi-tenant systems with HoRNDIS installed should only connect trusted USB devices to their system.} \\ 
\hline
\multicolumn{2}{|p{5cm}|}{Memory Read (Memory Errors)} & \textbf{Memory Read (Memory Errors):	7.3} \\ 
\hline
55 & \multicolumn{2}{p{13cm}|}{CVE-2020-4068:  In APNSwift 1.0.0, calling APNSwiftSigner.sign(digest:) is likely to result in a heap buffer overflow. This has been fixed in 1.0.1.} \\ 
\hline
\multicolumn{2}{|p{5cm}|}{Memory Read (Memory Errors)} & \textbf{Memory Read (Memory Errors):	9.26} \\ 
\hline
56 & \multicolumn{2}{p{13cm}|}{CVE-2020-15199:  In Tensorflow before version 2.3.1, the \`{}RaggedCountSparseOutput\`{} does not validate that the input arguments form a valid ragged tensor. In particular, there is no validation that the \`{}splits\`{} tensor has the minimum required number of elements. Code uses this quantity to initialize a different data structure. Since \`{}BatchedMap\`{} is equivalent to a vector, it needs to have at least one element to not be \`{}nullptr\`{}. If user passes a \`{}splits\`{} tensor that is empty or has exactly one element, we get a \`{}SIGABRT\`{} signal raised by the operating system.} \\ 
\hline
\multicolumn{2}{|p{5cm}|}{Memory Read (Memory Errors)} & \begin{tabular}[c]{@{}l@{}}Restart Or Reboot:	4.26\\\textbf{Memory Read (Memory Errors):	3.88}\end{tabular} \\ 
\hline

57 & \multicolumn{2}{p{13cm}|}{CVE-2020-11068:  In LoRaMac-node before 4.4.4, a reception buffer overflow can happen due to the received buffer size not being checked. This has been fixed in 4.4.4} \\ 
\hline

\multicolumn{2}{|p{5cm}|}{Memory Read (Memory Errors)} & \textbf{Memory Read (Memory Errors):	9.9} \\ 
\hline
58 & \multicolumn{2}{p{13cm}|}{CVE-2020-8649:  There is a use-after-free vulnerability in the Linux kernel through 5.5.2 in the vgacon\_invert\_region function in drivers/video/console/vgacon.c.} \\ 
\hline
\multicolumn{2}{|p{5cm}|}{Memory Read (Memory Errors)} & \textbf{Memory Read (Memory Errors):	9.44} \\ 
\hline
59 & \multicolumn{2}{p{13cm}|}{CVE-2020-12652:  The \_\_mptctl\_ioctl function in drivers/message/fusion/mptctl.c in the Linux kernel before 5.4.14 allows local users to hold an incorrect lock during the ioctl operation and trigger a race condition, i.e., a "double fetch" vulnerability, aka CID-28d76df18f0a. NOTE: the vendor states "The security impact of this bug is not as bad as it could have been because these operations are all privileged and root already has enormous destructive power."} \\ 
\hline
\multicolumn{2}{|p{5cm}|}{Memory Read (Memory Errors)} & \textbf{Memory Read (Memory Errors):	8.22} \\ 
\hline
60 & \multicolumn{2}{p{13cm}|}{CVE-2019-12660:  A vulnerability in the CLI of Cisco IOS XE Software could allow an authenticated, local attacker to write values to the underlying memory of an affected device. The vulnerability is due to improper input validation and authorization of specific commands that a user can execute within the CLI. An attacker could exploit this vulnerability by authenticating to an affected device and issuing a specific set of commands. A successful exploit could allow the attacker to modify the configuration of the device to cause it to be non-secure and abnormally functioning.} \\ 
\hline
\multicolumn{2}{|p{5cm}|}{Memory Modification (Memory Errors)} & \textbf{Memory Modification (Memory Errors):	10.97} \\ 
\hline
61 & \multicolumn{2}{p{13cm}|}{CVE-2019-13522:  An attacker could use a specially crafted project file to corrupt the memory and execute code under the privileges of the EZ PLC Editor Versions 1.8.41 and prior.} \\ 
\hline
\multicolumn{2}{|p{5cm}|}{Memory Modification (Memory Errors)} & \textbf{Memory Modification (Memory Errors):	11.15} \\ 
\hline
62 & \multicolumn{2}{p{13cm}|}{CVE-2018-10620:  AVEVA InduSoft Web Studio v8.1 and v8.1SP1, and InTouch Machine Edition v2017 8.1 and v2017 8.1 SP1 a remote user could send a carefully crafted packet to exploit a stack-based buffer overflow vulnerability during tag, alarm, or event related actions such as read and write, with potential for code to be executed.} \\ 
\hline
\multicolumn{2}{|p{5cm}|}{Memory Read (Memory Errors), Memory Modification (Memory  Errors)} & \begin{tabular}[c]{@{}l@{}}\textbf{Memory Read (Memory Errors):	4.84}\\\textbf{Memory Modification (Memory Errors):	1.84}\end{tabular} \\ 
\hline
63 & \multicolumn{2}{p{13cm}|}{CVE-2019-12660:  A vulnerability in the CLI of Cisco IOS XE Software could allow an authenticated, local attacker to write values to the underlying memory of an affected device. The vulnerability is due to improper input validation and authorization of specific commands that a user can execute within the CLI. An attacker could exploit this vulnerability by authenticating to an affected device and issuing a specific set of commands. A successful exploit could allow the attacker to modify the configuration of the device to cause it to be non-secure and abnormally functioning.} \\ 
\hline
\multicolumn{2}{|p{5cm}|}{ Memory Modification (Memory  Errors), Disable Protections} 
& \begin{tabular}[c]{@{}l@{}}\textbf{Memory Modification (Memory Errors):	10.97}\\\textbf{Disable Protections:	2.81}\end{tabular} \\ 
\hline
64 & \multicolumn{2}{p{13cm}|}{CVE-2018-15376:  A vulnerability in the embedded test subsystem of Cisco IOS Software for Cisco 800 Series Industrial Integrated Services Routers could allow an authenticated, local attacker to write arbitrary values to arbitrary locations in the memory space of an affected device. The vulnerability is due to the presence of certain test commands that were intended to be available only in internal development builds of the affected software. An attacker could exploit this vulnerability by using these commands on an affected device. A successful exploit could allow the attacker to write arbitrary values to arbitrary locations in the memory space of the affected device.} \\ 
\hline
\multicolumn{2}{|p{5cm}|}{Memory Modification (Memory Errors)} & \textbf{Memory Modification (Memory Errors):	11.77} \\ 
\hline
65 & \multicolumn{2}{p{13cm}|}{CVE-2019-1052:  A remote code execution vulnerability exists in the way that the Chakra scripting engine handles objects in memory in Microsoft Edge, aka 'Chakra Scripting Engine Memory Corruption Vulnerability'.} \\ 
\hline
\multicolumn{2}{|p{5cm}|}{Memory Read (Memory Errors)} & \textbf{Memory Read (Memory Errors):	10.11} \\ 
\hline
66 & \multicolumn{2}{p{13cm}|}{CVE-2020-3309:  A vulnerability in Cisco Firepower Device Manager (FDM) On-Box software could allow an authenticated, remote attacker to overwrite arbitrary files on the underlying operating system of an affected device. The vulnerability is due to improper input validation. An attacker could exploit this vulnerability by uploading a malicious file to an affected device. A successful exploit could allow the attacker to overwrite arbitrary files on as well as modify the underlying operating system of an affected device.} \\ 
\hline
\multicolumn{2}{|p{5cm}|}{Write To Existing File} & \textbf{Write To Existing File:	10.73} \\
% \bottomrule
\hline
\caption{The evaluation of classifying 66 CVE  into one or more functionalities based on only the description without considering the second input. The table shows the top K prediction for each CVE description where K equals to the total number of predictions until all the correct classes are predicted. The correct predictions are depicted by bold font.}
\label{tab: 66_eval}
\end{longtable}
\end{small}
