# Supplementary material for: CVE-driven Attack Technique Prediction with Semantic Information Extraction and a Domain-specific Language Model
Source: arXiv:2309.02785 source file (2023-09-06)
Supplement: Supplementary file 2 [file Appendix.tex]

% ------------------------------------------- Functionality Documentation
\iffalse
\subsection{Functionality Documentation}\label{sec: functionality}
MITRE guideline  has provided sixteen functionality names \footnote{\url{https://github.com/center-for-threat-informed-defense/attack_to_cve/blob/master/methodology.md}} without any 
We define sixteen different most common functions an attacker may be trying to gain access to through the exploitation known as functionalities. 
If $f_z$ denotes the functionality $f$ with index $z$, let's define the functionalities as follows :\\
{\scriptsize
\textbf{1) Create Account ($f_{z=1}$)}: the act of unauthorized creation of new accounts or adding new users to the victim system done by the attacker.
\\
\newline
\textbf{2) Create Or Upload File ($f_{z=2}$)}: the act of unauthorized creation or uploading any file to any system for any purpose done by the attacker.
\\
\newline
\textbf{3) Delete Files ($f_{z=3}$)}: the act of unauthorized deletion or destruction of any information including but not limited to files, contents, data, etc., done by the attacker. It is different from data manipulation.
\\
\newline
\textbf{4) Disable Protections ($f_{z=4}$)}: the act of causing any malfunction, interruption, or abnormality in any security/defensive process or system such as anti-viruses, anti-malware, authentication procedures, firewall, security checks, etc., done by the attacker.
\\
\newline
\textbf{5) Install App ($f_{z=5}$)}: the act of delivering and/or installing any malicious application or configuration on the victim's system causing further threats, done by the attacker.
\\
\newline
\textbf{6) Memory Modification (Memory Buffer Errors, Pointer Issues, Type Errors, etc.) ($f_{z=6}$)}: the act of any invalid modification, manipulation, and/or write to the memory (e.g., buffer, kernel, memory locations, pointers, etc.) leading to memory issues such as buffer-over read, memory crash, buffer overflow, etc., done by the attacker.
\\
\newline
\textbf{7) Password Reset ($f_{z=7}$)}: the act of manipulating an account such as modifying credentials (e.g., ID, username, password, email account name, etc.) for any purpose, done by the attacker.
\\
\newline
\textbf{8) Change Ownership or Permissions ($f_{z=8}$)}: the act of changing file ownership, and/or modifying access permission (access controls) for any purpose, done by the attacker.
\\
\newline
\textbf{9) Modify Configuration ($f_{z=9}$)}: the act of modifying, editing, and manipulating any systems configuration and/or settings causing further threats, done by the attacker.
\\
\newline

\textit{NOTE 1}: The actions and intention in "Install App" and "Modify Configuration" are quiet similar sharing similar techniques (not same), and since there is no ground truth available to distinguish them, we combine these two and considered them as a single functionality.\\
\newline
\textbf{10) Obtain Sensitive Information - Other Data ($f_{z=10}$)}: the act of obtaining any non-credential sensitive information without authorization via any method (unauthorized access to files, databases, memory, etc.) for any purpose, done by the attacker.
\newline
% \\\textit{NOTE 2}: Any action related to Read/Access can associate with one or more of the four above functionalities since they already share common MITRE Techniques.\\
\newline
\textbf{11) Obtain Sensitive Information - Credentials ($f_{z=11}$)}: the act of obtaining any user/system credentials without authorization via any method (unauthorized access to files, databases, memory, etc.) for any purpose, done by the attacker.
\\
\newline
\textbf{12) Read From Memory ($f_{z=12}$)}: the act of unauthorized reading any information or data from memory for any purpose, done by the attacker.
\\
\newline
\\\textit{NOTE 2}: "Obtain Sensitive Information - Other Data" and "Read From Memory" share exactly the same MITRE technique.  However, since the action and the purpose might differ, they are considered as separate functionalities.
\newline
 \textbf{13) Read Files ($f_{z=13}$)}: the act of unauthorized reading any information including from files, done by the attacker.
 \\
 \textit{NOTE 4}: This functionality and "Obtain Sensitive Information" (($f_{z=10}$) and ($f_{z=11}$))" are mainly using the "Read" action mentioned in the previous functionalities, hence they share mutual characteristics with each other in terms of common MITRE techniques.\\
\newline
\newline
\textbf{14) Memory Read (Memory Buffer Errors, Pointer Issues, Type Errors, etc.) ($f_{z=14}$)}: the act of any invalid reading from the memory (e.g., buffer, kernel, memory locations, pointers, etc.) leading to memory issues such as buffer-over read, memory crash, buffer overflow, etc., done by the attacker.
\\
\newline
\textbf{15) Restart Or Reboot ($f_{z=15}$)}: the act of crashing, shutting down, or rebooting any system often leading to a denial of services, done by the attacker.
\\
\newline
\textbf{16) Write To Existing File ($f_{z=16}$)}: the act of modifying the content of the existing file for any purpose, done by the attacker.

}
\begin{figure}[h]
\centering
\includegraphics[width=8cm]{Figs/functionality_rel.png}
\caption{Shows the functionalities and their relationships. In relationship definitions, 
The term "inheritance" denotes that the child's functionality inherits all of its parent's characteristics in addition to its own unique ones. The characteristics refer to the same threat action(s) and/or the same MITRE technique(s).
"commonality" on the other hand refers to the semantic similarity between two functionalities, but not necessarily the same behavior.}
\centering
\label{fig: functionality_rel}
\end{figure}

Fig. \ref{fig: functionality_rel} demonstrates all of the functionalities and their associated dependencies. We have defined two dependencies such as commonality and inheritance. The term "inheritance" denotes that the child's functionality inherits all of its parent's characteristics in addition to its own unique ones. The characteristics refer to the same threat action(s) and/or the same MITRE technique(s) the functionalities associated with. For example, to conduct \textit{out-of-bound-read}, which is associated with functionality "$f_{z=14}$: Memory Read (Memory Errors)", an attacker must conduct the \textit{read} action which is also associated with functionality "$f_{z=12}$: Read From Memory", such as \textit{reading arbitrary memory} or \textit{reading kernel memory}.
On the other hand, commonality refers to the semantic similarity of two classes which means both classes can describe similar impacts or actions, but not necessarily the same. If the commonality is strong, it implies that the impact can be the same and in some cases cannot be differentiated. For example, an attacker can install an extension ($f_z=$ 5) and manipulate the system configuration ($f_z=$ 9), or an attacker can read memory locations ($f_z=$ 14) and gain sensitive information ($f_z=$ 10). In other words, the actions or the impact can be used interchangeably for both classes. On the other hand, when the commonality is weak, a single action or impact can imply two different concepts. For example, when an attacker gains sensitive information, this can be the list of system files ($f_z=10$ ), and in the meantime, it can be the plain-text password ($f_z=11$). 
Notably, action or impact refers to the same concept using a different language in strong commonality, but in weak commonality, action or impact refers to a distinct concept using the same language. According to the table, types 13 and 14 are the children of type 12 (inheritance), type 10 and 11, and 10 and 12 have strong commonality dependency, type 5 and 9 also have strong commonality, and type 10 and 11 have weak commonality dependency. Since types 13 and 14 are inherited from class 12, they have a strong commonality with classes 10 and 11 as well. Such dependencies are critical in corpus generation, dataset creation, and also in model training and evaluation. To summarize, if $f_z$ and $f_z'$ represent two functionalities and $R(f_z, f_z')$ demonstrates the dependency between them:
\newcommand{\eqsize}{\relsize{-1}}
\begin{align*}

    \eqsize R(f_z, f_{z'}) &= \textit{Inher} && \text{IF $f_{z'}$ is the inheritor of $f_z$} \\
    \eqsize R(f_z, f_{z'}) &= \textit{Strong} && \text{IF $f_z$ and $f_{z'}$ have strong} \\
    &&& \text{commonality dependency} \\
    \eqsize R(f_z, f_{z'}) &= \textit{Weak} && \text{IF $f_z$ and $f_{z'}$ have weak} \\
    &&& \text{commonality dependency} \\
    \eqsize R(f_{z'}, f_{z''}) &= \textit{Strong} && \text{IF }  R(f_z, f_{z'}) = \textit{Inher} \quad \text{and} \quad R(f_z, f_{z''}) = \textit{Strong}
\end{align*}



Each of the preceding functionality refers to a specific malicious action carried out by an attacker in order to compromise a system. 
Specifying the dependencies helps in better understanding and processing the main concept of each functionality leading to strategic text extraction and annotation, discussed in the next section.
% -------------------------------------------
% ------------------------------------------- EXTRACTOR
% -------------------------------------------
\iffalse
\subsection{EXTRACTOR}\label{chapter:EXTRACTOR}
EXTRACTOR \cite{satvat2021extractor}  is an off-the-shelf tool that leverages SRL to extract threat actions from the technical text reports in the form of a graph. 
SRL can assign semantic labels to phrases and words in a sentence, where each label specifies the semantic role that each phrase or word plays in the sentence in association with the predicate or verb of the sentence. In SRL, the tags assigned to sentence components are called arguments (denoted by ARG).
Table \ref{tab: propbank} shows these arguments and the definition based on PropBank \cite{palmer2005proposition}.

EXTRACTOR operates by performing different rounds of transformations on the text to bring it from a highly complex and potentially ambiguous form to a simpler form. This simplified text is further processed to obtain a provenance graph that can be successfully used for threat detection.
Fig. \ref{fig: EXTRACTOR_ow} shows the four major components that the EXTRACTOR is composed of including text normalization, resolution, summarization, and graph generation.
\begin{figure}[h]
\includegraphics[width=11cm]{Figs/EXTRACTOR_ow.png}
\caption{The overview of EXTRACTOR framework}
\centering
\label{fig: EXTRACTOR_ow}
\end{figure}

Similar works mostly consider limited resources, such as sample malware or limited types of security reports, to extract threat actions. On the other hand,  they focused on exchanging IOCs\footnote{Indicator of Compromise} than describing how those IOCs are connected and how the attacks behave. 
The main advantage of EXTRACTOR compared to similar works is that it focuses on extracting the attack behavior and captures system-level causality in the form of provenance graphs and utilizes the public CTI reports to convert raw text into actionable knowledge. Furthermore, the different rounds of transformations enable the EXTRACTOR to deliver clean, concise, and fine-grain threat actions that can be used directly to represent functionalities. Therefore, we customized EXTRACTOR based on a particular set of linguistic rules in this work in order to extract set if threat actions from cybersecurity text to build a solid and precise dataset.

% Normalization
Normalization is responsible for an initial round of sentence simplification and transformation to a canonical form by breaking long and complex sentences into shorter sentences, which is easier to process. Normalization is comprised of tokenization, homogenization, and conversion. These steps perform the detection of sentence boundaries, and word homogenization in which multiple textual representations of the
same concept are replaced by the same textual representation (e.g., C2, C\&C, and Command and
Control are different representations of the same entity, while verbs like stores and saves may represent an action that corresponds to a write system call), and passive-to-active verb conversion. 

% Resolution
The resolution resolves ambiguities in the sentences reconciling implicit references that refer to the same entity into the actual referent. This phase comprises three components as Ellipsis Subject Resolution (ESR), Pronoun Resolution (PR), and Entity Resolution (ER). 

Ellipsis subject is a linguistic structure where a sentence's subject is not present that confuses the state-of-the-art NLP toolkits, thus resulting in the loss of the narrative sequence and the story relationships. ESR module utilizes POS and DP to detect target sentences, builds a list of candidate subjects among the entities appearing in the sentences preceding the current sentence, and then picks the most probable candidates from the list based on the distance of that candidate from the sentence with the missing subject.

PR is the process by which pronouns are mapped and substituted to the antecedent entities that they refer to. Processing documents (building a provenance graph) without PR can result in the appearance of several nodes (i.e., pronouns) for a single entity. To resolve pronouns, EXTRACTOR adapts a popular coreference resolution model, NeuralCoref\footnote{https://github.com/huggingface/neuralcoref}.

ER is the process by which noun or verb phrases that refer to another entity inside the same sentence are substituted by that entity or are eliminated as redundant focusing on actionable entities and actions that are likely to appear in audit logs, using POS tagging and DP with domain knowledge contained in CTI nouns dictionary or in a corpus of common phrases. For example, phrases like \textit{"tries to open} and \textit{"makes the modification"} will be converted to \textit{"open"} and \textit{"modify"}, respectively, using this component.
% Summarization
Summarization removes the portion of text that is not strictly related to the attack behavior, and that cannot be observed in the logs. Ideally, only the sentences that describe actions that may be observed in the audit logs should be preserved. For summarization, EXTRACTOR takes advantage of a two-step approach to deal with sentence verbosity and word verbosity using the BERT classifier and BiLSTM network. For sentence verbosity, they labeled $8,000$ threat sentences under two classes of productive and nonproductive and trained BERT on this set. Word verbosity removes unnecessary words from the productive sentences that it receives as input from BERT using the BiLSTM model and a word remover component. After a sentence is processed by a BiLSTM network, its components are tagged as \textit{Agent}, \textit{Patient}, and \textit{Action}, and other types of arguments. For this component, EXTRACTOR utilizes System Entity Extractor (SEE) in which, a sentence component that is tagged for removal will be removed if it does not contain any entities that can be generated by the rules of the SEE component.

% Graph Generation
Finally, Graph Generation is responsible for resolving the temporal and causal order among the events in the text and for building the final provenance graph (this component addresses the Relationships Extraction challenge)

Some of the EXTRACTOR components may be assisted by a set of dictionaries that contain terms related to CTI language (relying on domain-specific dictionaries of concepts is a common approach in many knowledge-based NLP systems.

In particular, EXTRACTOR uses two dictionaries. First, a system call synonym dictionary, which contains verbs representing system calls (e.g., write, fork) and their corresponding synonyms.
These synonyms represent the possible verbs that can be used in CTI reports and very likely refer to a system call. 
Second, the CTI nouns dictionary contains noun phrases commonly used in CTI reports, as well as different textual representations of the same concept. The former contains 87 verbs representing system calls, while the latter holds over 1112 common noun phrases in the CTI report.
\fi
\fi
